# Supplementary material for: Open-Vocabulary Functional 3D Scene Graphs for Real-World Indoor Spaces
Source: arXiv:2503.19199 source file (2025-03-24)
Supplement: Supplementary file 1 [file X_suppl.tex]

\section{Details in the Method}
\subsection{Confidence-Aware Remote Reasoning}

\begin{figure*}[t]
    \centering
\includegraphics[width=0.99\textwidth]{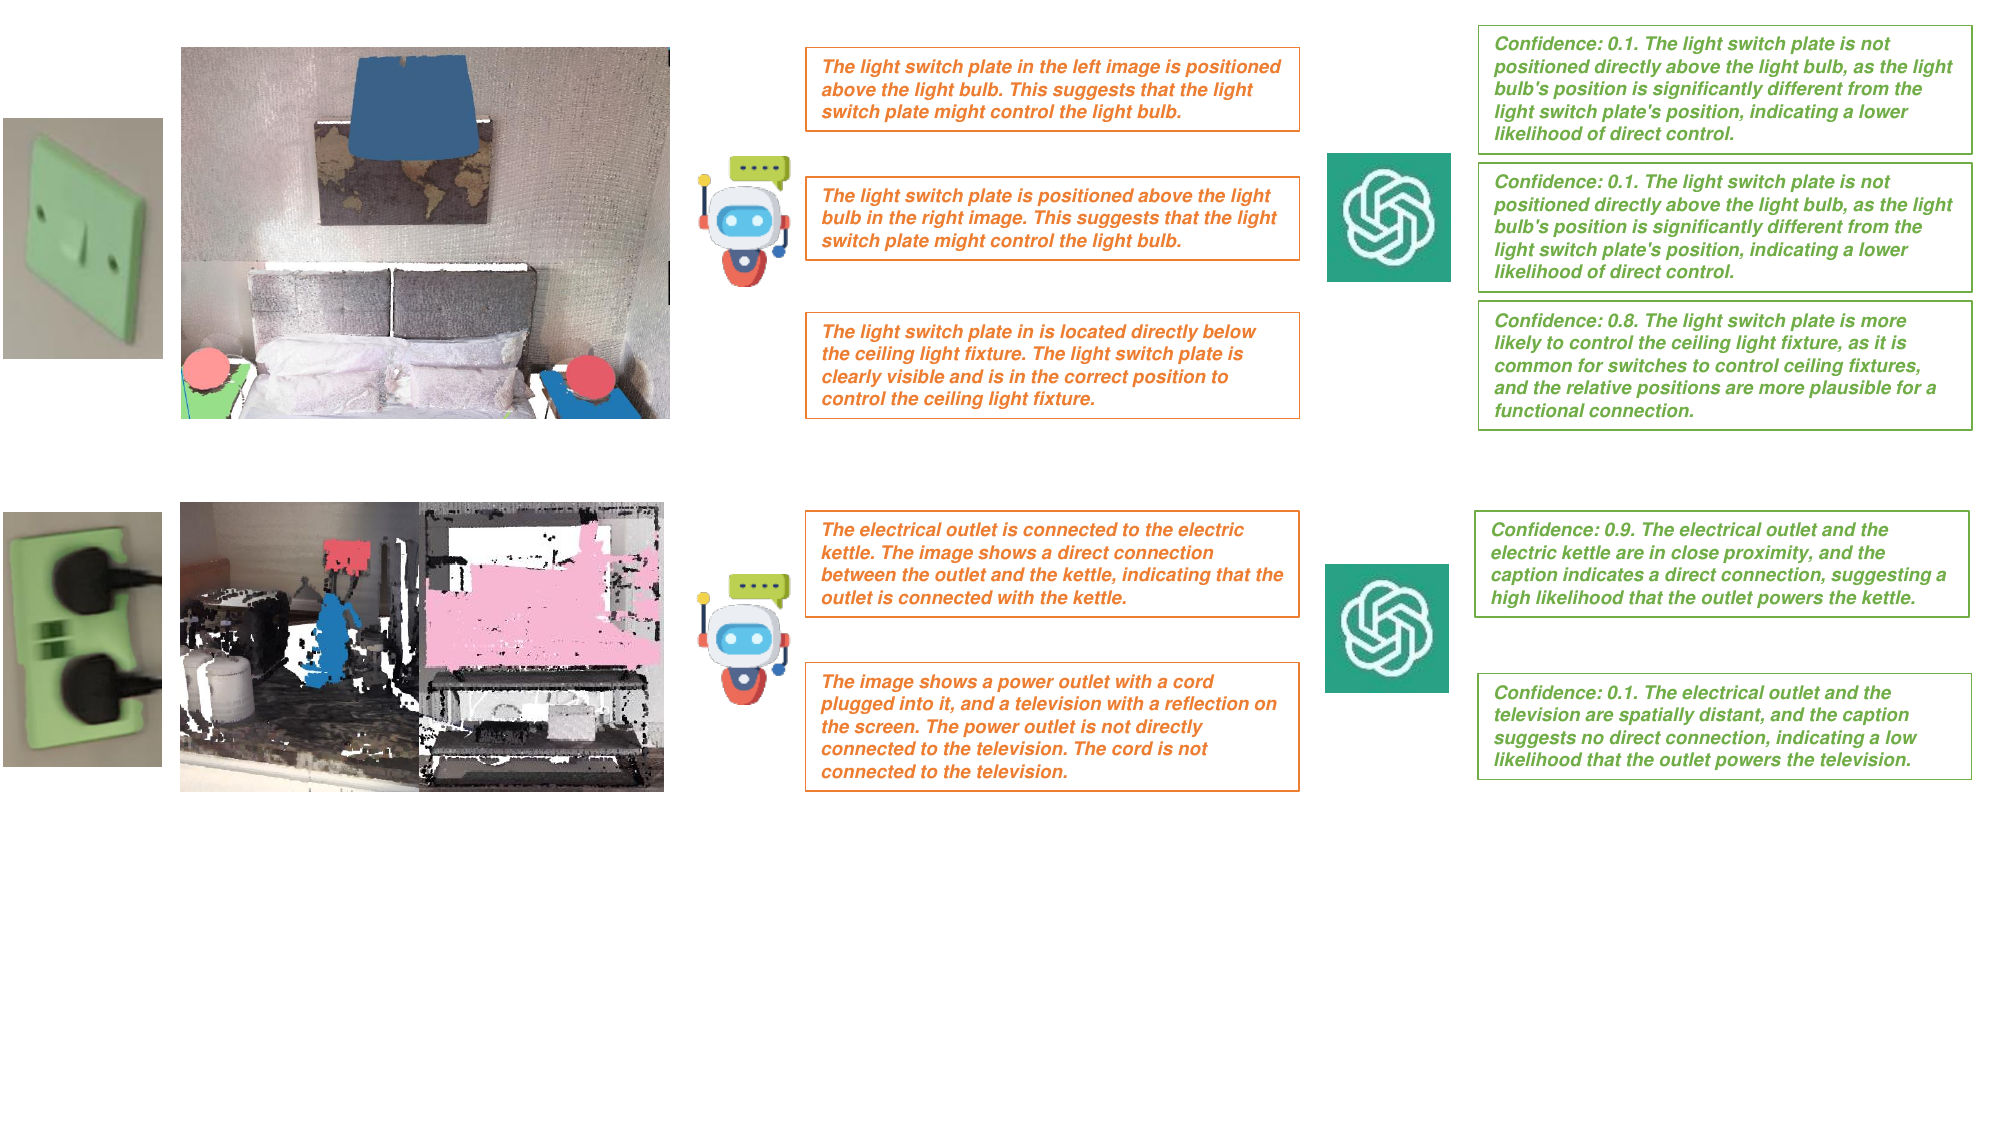}
    \caption{Illustration of the confidence-aware remote relationship reasoning.}
    \label{fig:remote}
\end{figure*}

In Section 4.3 of the main paper, we introduce the methodology of confidence-aware remote relationship reasoning. Here, we provide two additional qualitative examples (see Figure~\ref{fig:remote}) to demonstrate both the process and the effectiveness of the proposed strategy in handling complex spatial relationships with confidence-aware reasoning.

In the first example, the remote relationship between the light switch and the ceiling light is identified as the most confident. The Vision-Language Model (VLM) first evaluates the feasibility by focusing on the relative layouts, concluding that “the light switch is in the correct position to control the ceiling light fixture.” The Large Language Model (LLM) then integrates all three feasibility descriptions into a global context, summarizing that “the light switch is more likely to control the ceiling light, as it is common for switches to control ceiling fixtures, and the relative positions are more plausible for a functional connection.”

In the second example, the VLM directly observes that the kettle is plugged into the electric outlet and asserts that “the outlet is connected with the kettle.” In contrast, it determines that the television is not connected to either the power outlet or the cord. Based on these observations, the LLM synthesizes the confidence results, summarizing that “the outlet and the kettle are in close proximity,” and assigns high confidence to this relationship.

\subsection{Other Implementation Details}

We provide additional implementation details of our method, OpenFunGraph, in this section. 
In the node candidate description, the $N_v$ we implement is 9, and we discard candidates that share fewer than $N_v$ multi-views to ensure robustness in the multi-view summary. All experiments are conducted on a single NVIDIA 3090 GPU, primarily utilized for RAM++, GroundingDINO, and LLAVA inference. 
For a typical scene composed of 200 frames, the OpenFunGraph pipeline takes approximately 20 minutes to process. This includes 11 minutes for candidate detection (10 minutes) and fusion (1 minute), 8 minutes for LLAVA processes, and 1 minute for GPT-4 inference.

\begin{figure*}[t]
    \centering
\includegraphics[width=0.99\textwidth]{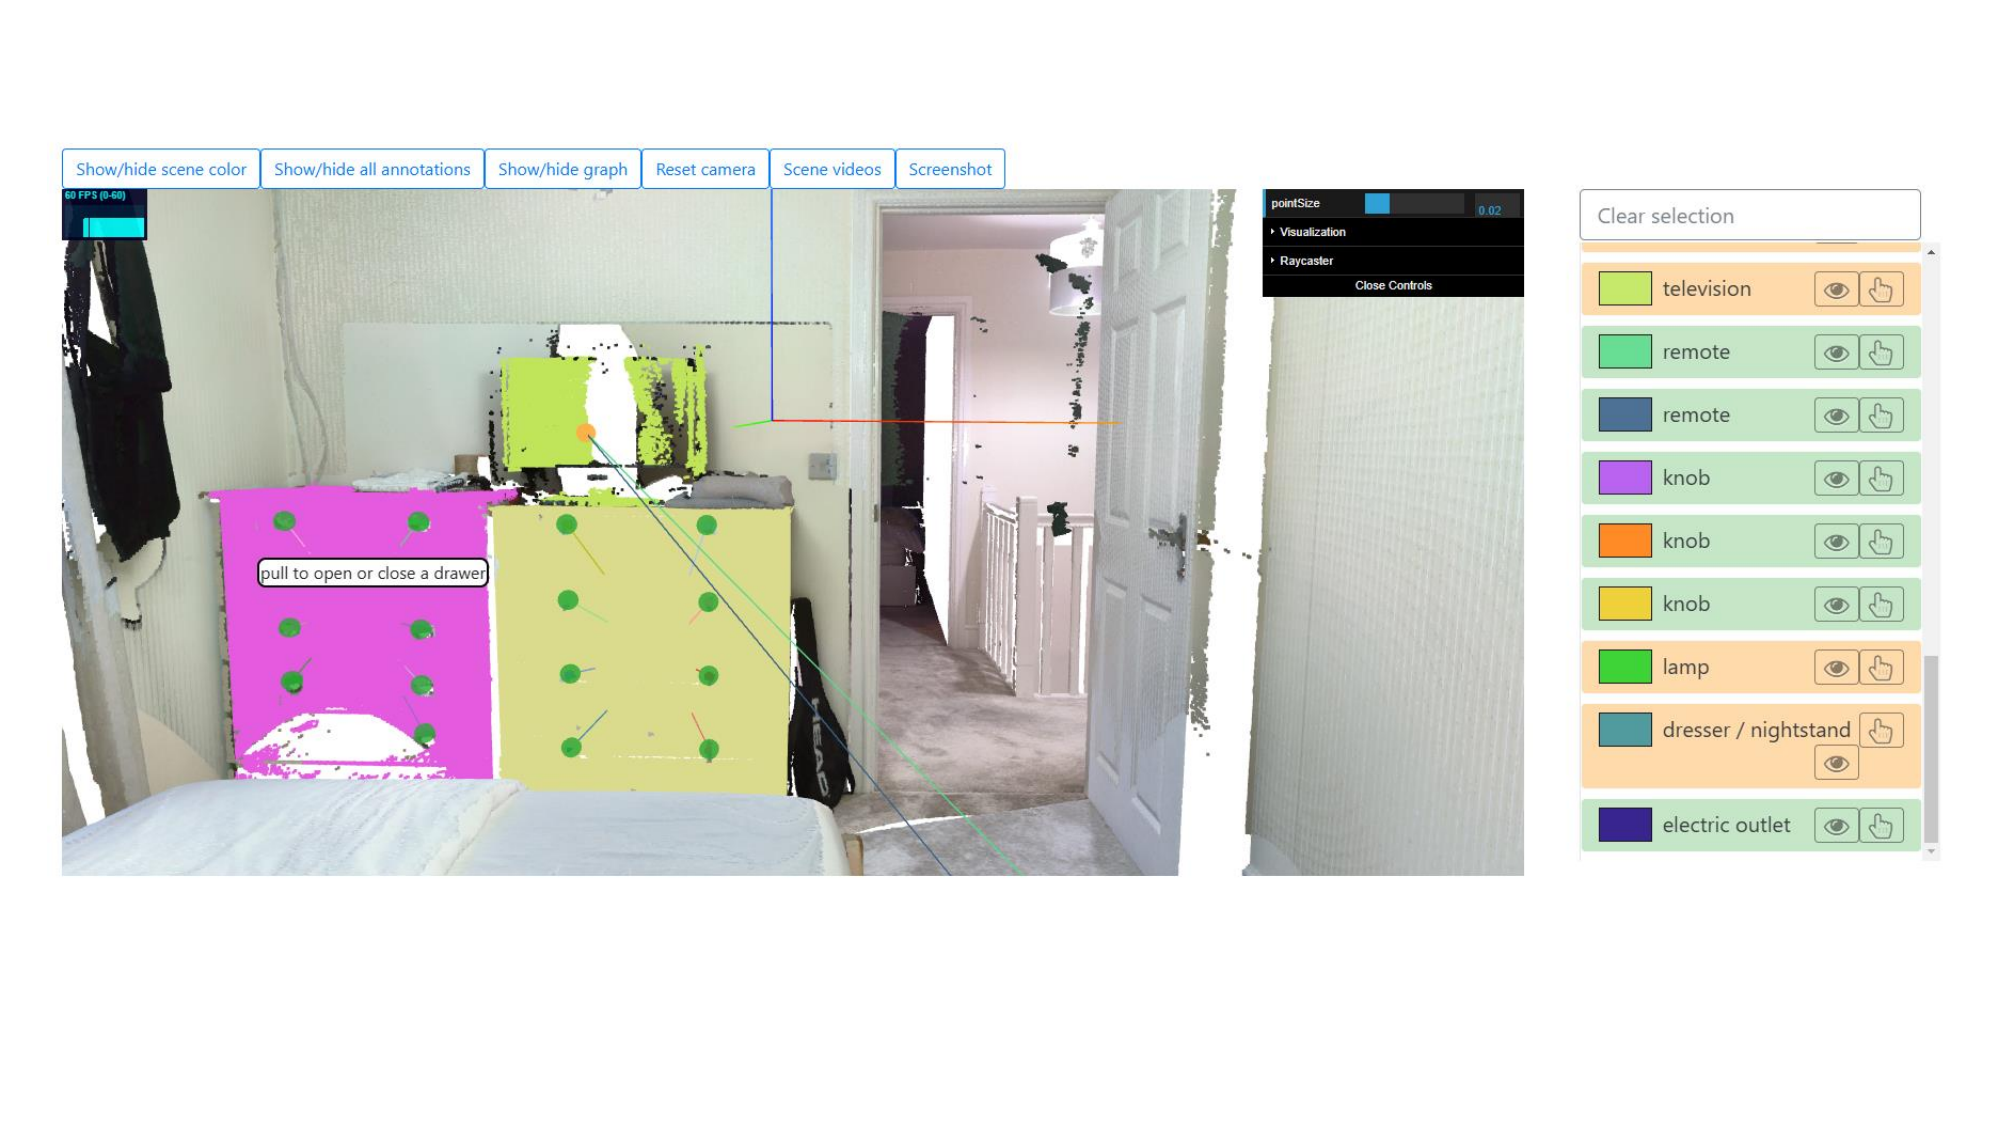}
    \caption{Our developed annotation tool for functional 3D scene graphs.}
    \label{fig:annotool}
\end{figure*}

\section{The Developed Annotation Tool}

As introduced in Section 5 of the main manuscript, we developed an annotation tool for creating functional 3D scene graph annotations in the SceneFun3D and our proposed FunGraph3D datasets. 
The designs of the tool are showcased in Figure~\ref{fig:annotool}. Annotators can navigate the 3D scene and annotate instances of objects and interactive elements with a free-form label. They are also required to connect each interactive element to the corresponding object it controls and provide a description of their relationship. 
To assist in the annotation process, annotators can view iPad videos or egocentric human-scene interaction videos captured during data collection. These videos provide additional context, enabling annotators to identify objects, functional elements, and their relationships more accurately and efficiently.

\section{Additional Ablation Studies}

\begin{table}[t!]
\centering
\resizebox{\linewidth}{!}{
\begin{tabular}{llccccc}
\toprule
 && \multicolumn{2}{c}{\textbf{Overall Nodes}} && \multicolumn{2}{c}{\textbf{Overall Triplets}}\\
\cline{3-4} \cline{6-7}
& \textbf{Experiments} & R@3 & R@10 && R@5 & R@10 \\
\hline
& LLAVA v1.6 $\rightarrow$ v0 & $48.6$ & $71.2$ && $36.3$ & $47.0$\\
& GPT v4 $\rightarrow$ v3.5   & $51.5$ & $65.7$ && $31.5$ & $45.0$\\
& Ours                        & $\mathbf{73.0}$ & $\mathbf{82.8}$ && $\mathbf{60.4}$ &$\mathbf{70.3}$\\
\midrule
& LLAVA v1.6 $\rightarrow$ v0 & $38.3$ & $53.8$ && $22.3$ & $29.1$\\
& GPT v4 $\rightarrow$ v3.5   & $41.4$ & $49.3$ && $18.1$ & $23.3$\\
& Ours                        & $\mathbf{55.5}$ & $\mathbf{65.8}$ && $\mathbf{29.8}$ & $\mathbf{45.0}$\\
\bottomrule
\end{tabular}
}
\caption{Ablation study for the foundation models on SceneFun3D \cite{delitzas2024scenefun3d} (Top) and our \datasetname{} (Bottom).}
\label{tab:extra_ablation}
\end{table}

We ablate different versions of the foundation models used, \ie, the VLM and the LLM, to evaluate how their capabilities affect the understanding of indoor functional relationships, as shown in Table~\ref{tab:extra_ablation}. 
A higher version of the VLM notably enhances node recognition, while improvements in the LLM substantially boost both triplet prediction and node recognition. This is achieved by strengthening the LLM's understanding of indoor functionalities and its responsiveness to prompts.

\section{Limitations}
The proposed pipeline relies on a 2D-based method due to limitations in 3D models' ability to accurately understand and localize small interactive elements, as illustrated by \cite{delitzas2024scenefun3d}. With advancements in 3D models, we aim to develop a fully 3D-based functional scene graph inference method in the future.

Additionally, due to resource constraints, the developed dataset is currently limited in scale, which restricts adaptive training for functional scene graph construction. We plan to significantly expand the dataset to address this limitation and support more robust and scalable training.
